# Supplementary material for: Low Curie-temperature ferromagnetic phase in SmPt2Cd20 possibly accompanied by strong quantum fluctuations
Source: arXiv:1706.02872 source file (2017-06-09)
Supplement: Supplementary file 1 [file Supplementary_Material.pdf]

Supplementary Material for “Low Curie-temperature ferromagnetic phase in $SmPt_2Cd_{20}$ possibly accompanied by strong quantum fluctuations” by A. Yamada *et al.*

## Magnetization

Magnetization $M(T)$ of $SmPt_2Cd_{20}$ can be estimated from the specific heat $C$ data using the following thermodynamic relation:

$$\left.\frac{\partial^2 M}{\partial T^2}\right|_H = \left.\frac{1}{T}\frac{\partial C}{\partial H}\right|_T . \tag{S1.1}$$

Figure S1 (a) shows $\Delta C(T) = C\,(T, 0.1\ \mathrm{T}) - C\,(T, 0\ \mathrm{T})$ obtained from the data shown in Fig. 3. $\Delta C(T)$ exhibits a sign change at $T_c' = 0.70$ K, i.e., $\Delta C < 0$ in $T < T_C'$ and $\Delta C > 0$ in $T > T_C'$. This is a typical behavior characteristic for a ferromagnetic transition. The slightly larger value of $T_C'$ as compared with $T_C = 0.64$ K corresponds to the shift of the specific heat peak in applied fields. Magnetization $M(T)$ evaluated using the following integrated equation

$$M(T) = \int_{T_m}^{T}\left[\int_{T_m}^{T'}\frac{1}{T''}\frac{\Delta C(T'')}{\Delta H}dT''\right]dT' + aT + b \tag{S1.2}$$

was shown in Fig. S1 (b). In eq. (S1.2), $T_m = 0.26$ K is the lowest temperature of the specific heat measurement and the constants $a$ and $b$ were determined so that the calculated $M(T)$ is consistent with the magnetization data shown in Fig.2. Below 1 K, $M(T)$ shows a sharp increase and a saturating behavior below $T_C'$. This behavior shows clearly that the ordering is of a ferromagnetic type.

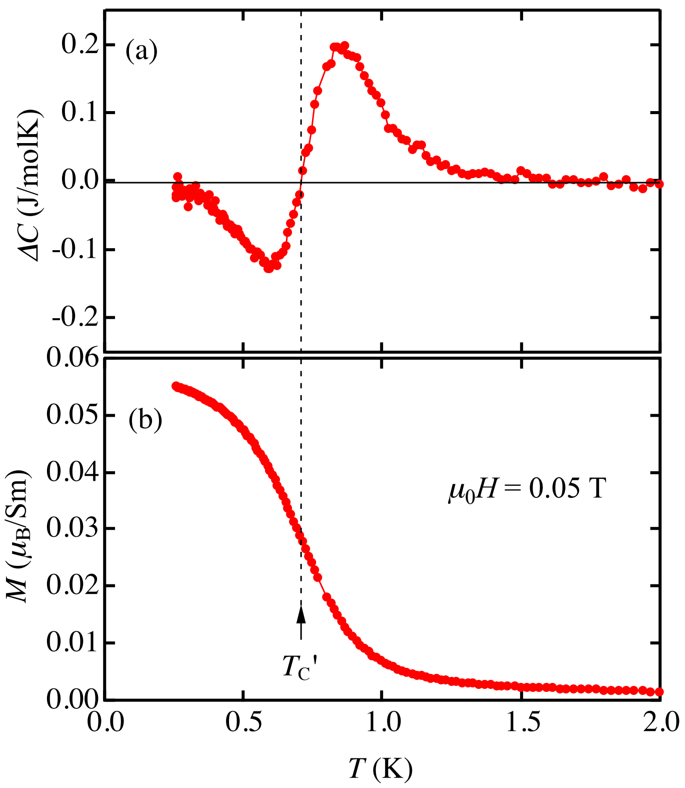


Figure S1: (a) the difference in specific heat $\Delta C(T) = C\ (T, 0.1\ \text{T}) - C\ (T, 0\ \text{T})$ and (b) the magnetization $M(T)$ calculated following the thermodynamic relation of eq. (S1.2) The arrow indicates the sign change in $\Delta C(T)$ at $T_C' = 0.70$ K.

## Magnetoresistance

Magnetoresistance (MR) of $SmPt_2Cd_{20}$ has been measured using a Helium-3 cryostat combined with a PPMS (Quantum Design) up to 9 T down to 0.5 K. The results are shown in Fig. S2. MR is always positive and is approximately proportional to $H^2$ over the investigated temperature range. This behavior is completely different from those observed in the usual ferromagnetic materials (e.g., Ni and Gd), which show negative MR (suppression of conduction electron scattering by FM fluctuations) that can be explained by theoretical calculations (for example, see Fig. 1 of Ref. [S1]). The temperature dependence of $\Delta\rho(9\ \text{T})/\rho(0\ \text{T})$ of $SmPt_2Cd_{20}$ is of the order of $10^{-2}$ and is extremely weak, showing no noticeable anomalies crossing $T_C$. These behaviors indicate that MR due to the cyclotron motion of conduction electrons dominates over

magnetic scatterings. A slight downward curvature appearing in $\Delta\rho(H)/\rho(0\ \mathrm{T})$ vs $H^2$ (see Fig. S2 (b)) may indicate contributions from field-dependent suppression of conduction electron scattering by FM fluctuations.

Studies of de Haas van Alphen effect have clarified that the Fermi surface consists of multibands in $R\mathrm{Ti_2Al_{20}}$ [S2]. Considering this fact, it is possible that $\mathrm{SmPt_2Cd_{20}}$ also has multibands and the dominant conduction band governing the transport properties is coupled extremely weakly with Sm 4*f* magnetic moments.

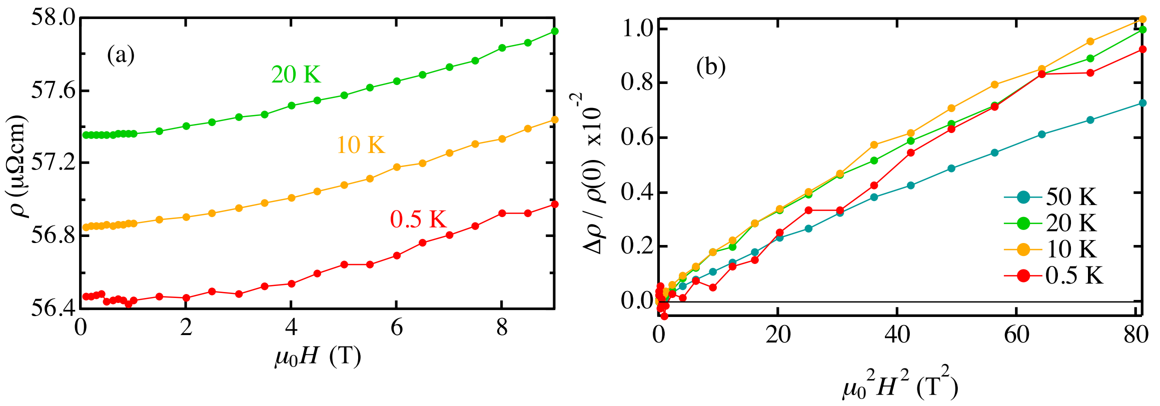


Figure S2 (a) transverse magnetoresistance of $\mathrm{SmPt_2Cd_{20}}$ measured with $I$ || [110] and $H$ || [1-11] and (b) $\Delta\rho(H)/\rho(0\ \mathrm{T})$ vs $H^2$ at 0.5, 10, 20, and 50 K.

References

[S1] I. Balberg, Physica B **91**, 71 (1977).

[S2] S. Nagashima, T. Nishiwaki, A. Otani, M. Sakoda, E. Matsuoka, H. Harima, and H. Sugawara, JPS Conf. Proc. **3**, 011019 (2014).
